# Supplementary material for: Robust Dialog State Tracking for Large Ontologies
Source: arXiv:1605.02130 source file (2016-05-07)
Supplement: Supplementary file 1 [file appendix.tex]

\section*{Appendix}
\addcontentsline{toc}{section}{Appendix}
TODO
